# Supplementary material for: Efficient Vertex-Oriented Polytopic Projection for Web-scale Applications
Source: arXiv:2103.05277 source file (2022-01-06)
Supplement: Supplementary file 1 [file dgap.tex]

\section{Duality gap bound}
\label{app:dgap}

Describe the duality gap bound derivation for the special class of problems.

%\subsection{Simple baselines}
%\label{subsec:qa_simbaseline}
{\bf Simple baselines}
In real applications it is important to evaluate the quality of the solution produced by an optimization algorithm against a simple and intuitive baseline. Very often, it is a greedy allocation algorithm with a set of business rules that ensure the constraints are satisfied. For example, for item matching problems the greedy solution would pick the best item with sufficient remaining budget and update the budget in real time. We show this baseline in figure~\ref{fig:qa_duality_gap}. The duality gap that characterizes the maximum unrealized improvement is contextualized in a comparison with the gain over the baseline.

\begin{figure}[ht]
%\vskip 0.2in
\begin{center}
\centerline{\includegraphics[width=0.7\columnwidth, clip]{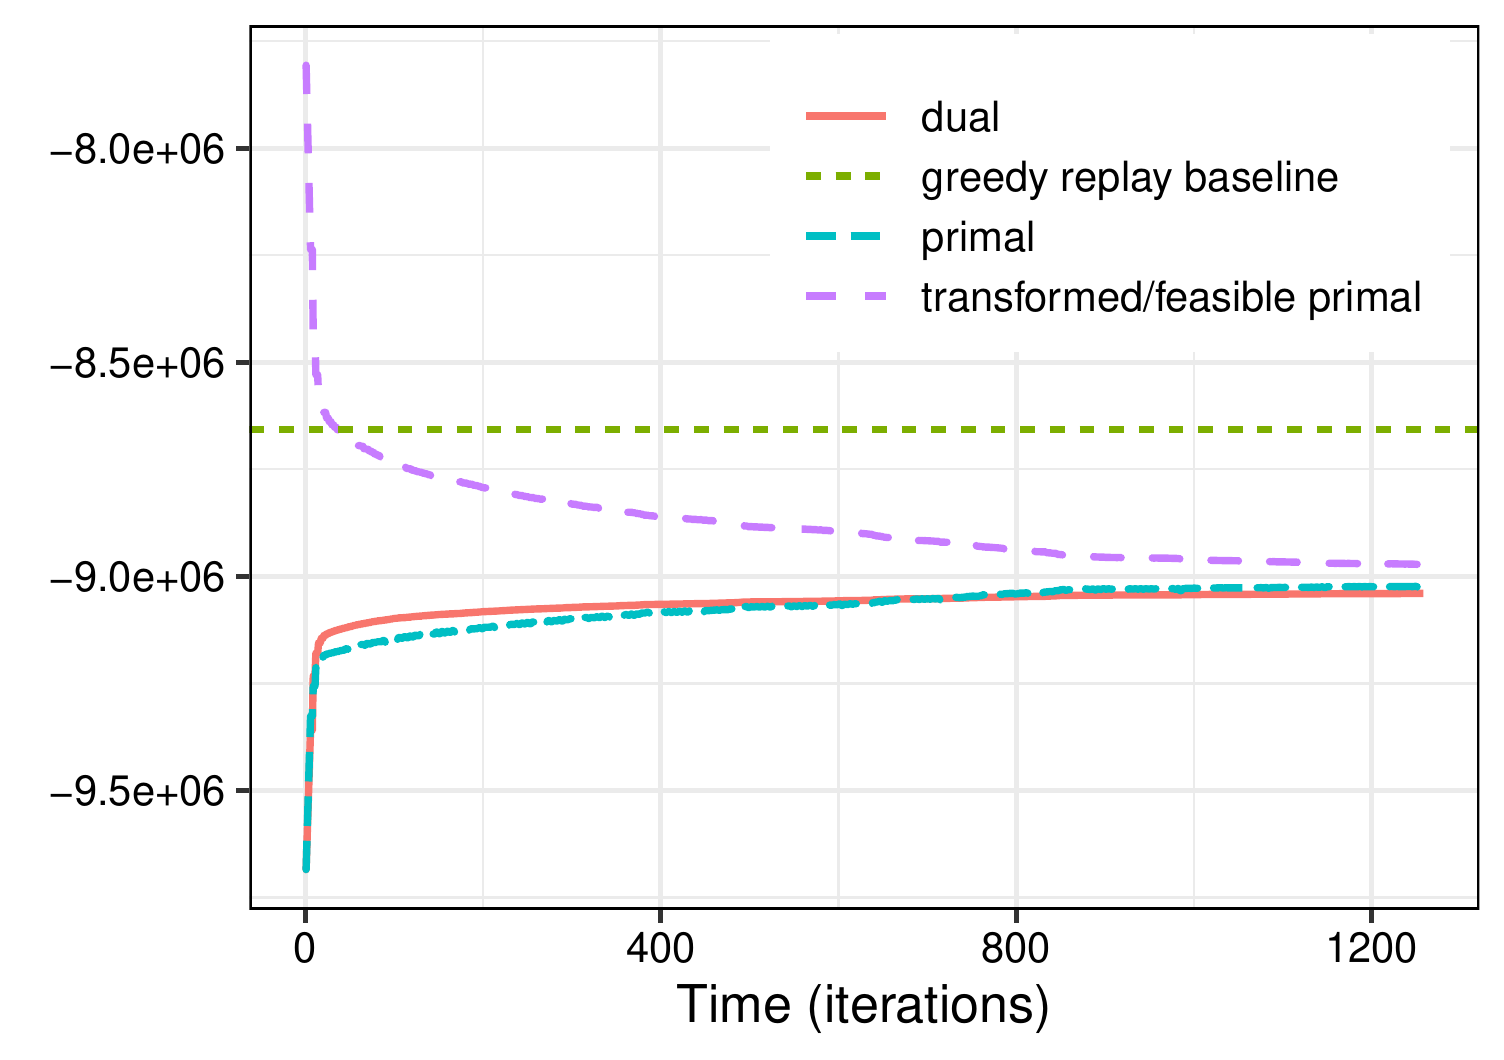}}
\caption{Visualization of the quality of the solution. The gap between dual and primal at transformed/feasible $x$ allows to estimate the potential of further objective improvement. The greedy baseline gives a reference point for estimating the magnitude of the gap. The baseline is built using using a greedy replay algorithm: each impression is assigned the best item with sufficient budget left, the budgets updated in real time.}
\label{fig:qa_duality_gap}
\end{center}
%\vskip -0.2in
\end{figure}
