# Supplementary material for: Efficient Vertex-Oriented Polytopic Projection for Web-scale Applications
Source: arXiv:2103.05277 source file (2022-01-06)
Supplement: Supplementary file 2 [file experiments.tex]

\section{Experiments}
\label{app:experiments}

\vspace{-0.2cm}

%Let us now turn to evaluating the quality of the methods.
A common method to evaluate the quality of the solution is to use toy datasets with a known solution to report duality gap. Our implementation\footnote{We will open-source the code upon publication. Some datasets would also be provided in the supplementary materials.} provides many such datasets of varying sizes to show the convergence of \dlip to retrieve the exact solution. However, in real-world internet marketplaces, often times retrieving a primal feasible solution (and hence duality gap) is non trivial.  Consider the ideal normalized quality score, $(g_0(\lambda) - g_0(0)) / (g_0(\lambda_0) - g_0(0))$. Since $g_0(\lambda_0)$ is unavailable, for sake of practicality we can replace it with $\gtil_0$, the best $g_0$ value obtained by the stage-wise $\gamma$ tuning method after a large number of iterations in stage 3. Thus, we evaluate methods using the quality score
\begin{equation}
  Q(\lambda) = 
  %\frac{(\gbest - g_0(\lambda))}{(\gbest - g_0(0))}
  \frac{g_0(\lambda) - g_0(0)} {\gtil_0 - g_0(0)}
  \label{eq:quality}
\end{equation}
Note that $Q(\lambda)\le 1$ for all methods. For practical goodness, we want to reach a $\lambda$ with $Q(\lambda)>0.999$.\footnote{A value of $Q(\lambda)=0.99$ is ``1\% off from the best'' and $0.9$ is ``10\% off from the best'' and so on.} To show this reaching clearly, we show all plots with a non-linearly scaled $Q$, but with the axis marked in terms of the actual $Q$ values.

We begin by comparing the optimizers discussed in \S\ref{subsec:costprofiling} (see Figure~\ref{fig:opt-results}).
AGD with fixed step size (a method used by \ecl) is very slow and hence it is not shown.
Improved AGD (with dynamic step size computation based on history and $L$) works much better, but it introduces a few hyperparameters that need tuning. Additionally, in all real datasets, the oscillations of $g_{\gamma}$ makes it hard to find the true optimal. 
Since LBFGS-B and PGA are proper ascent methods, it is easier to terminate their solution.
Across all applications, we observe that LBFGS-B is the fastest optimizer. PGA is considerably slower. 

%\vskip -0.1in
\begin{figure}[h]
    \centering
    \includegraphics[width=0.6\columnwidth]{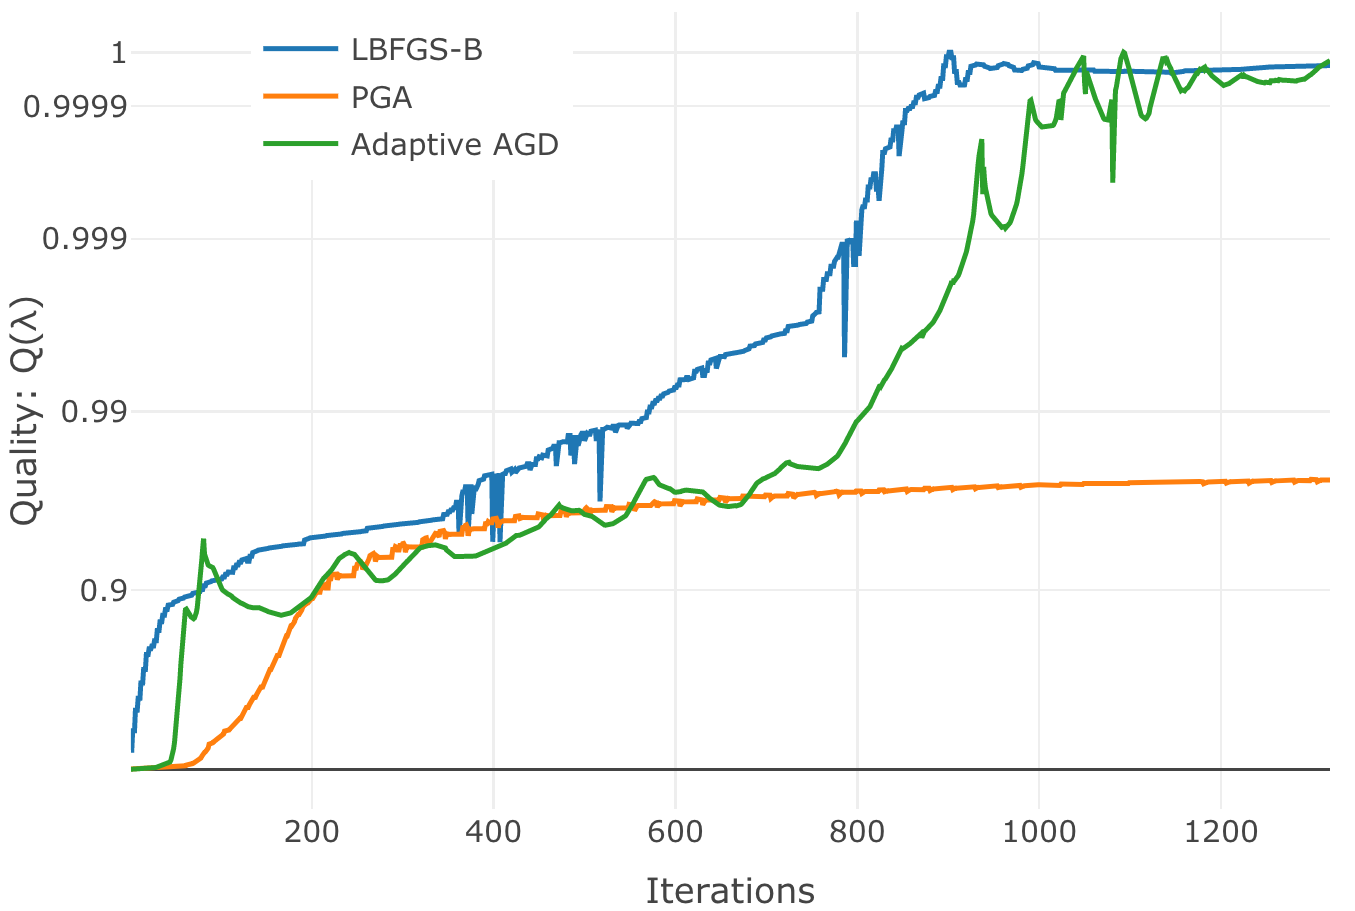}
    %\vspace{-0.2cm}
    \caption{The effect of the optimization algorithm on $Q(\lambda)$}
    \label{fig:opt-results}
%\vskip -0.1in
\end{figure}

% \begin{table}[!ht]
% \centering
% \begin{tabularx}{0.9\linewidth} { 
%     >{\centering\arraybackslash}X
%   | >{\centering\arraybackslash}X
%   | >{\centering\arraybackslash}X 
%   | >{\raggedleft\arraybackslash}X  }
% \hline
% \multirow{2}{*}{Method} & \multicolumn{3}{c}{$D_1$}                        \\
%                         & \multicolumn{1}{c}{50} &
%                         \multicolumn{1}{c}{100} & \multicolumn{1}{c}{500}  \\
% \hline
% \ecl  &  0.0356 & 0.0777 & 0.4496 \\
% \dlip  & 0.8774 & 0.9087 & 0.9788  \\
% \hline
% \end{tabularx}

% \begin{tabularx}{0.9\linewidth} { 
%     >{\centering\arraybackslash}X
%   | >{\centering\arraybackslash}X
%   | >{\centering\arraybackslash}X
%   | >{\centering\arraybackslash}X 
%   | >{\raggedleft\arraybackslash}X  }
% \hline
% \multirow{2}{*}{Method} & \multicolumn{4}{c}{$D_2$}                         \\
%                         & \multicolumn{1}{c}{500} &
%                         \multicolumn{1}{c}{500} & \multicolumn{1}{c}{1000} & \multicolumn{1}{c}{5000} 
%                         \\
% \hline
% \ecl    & 0.0006 & 0.0242 & 0.0744 & 0.6664 \\
% \dlip   & 0.9216 & 0.9719 & 0.9870 & 0.9984  \\
% \hline
% \end{tabularx}
% \caption{Quality of solution, $Q(\lambda)$, when operating on a time budget.}
% \label{tab:quality-results}
% \end{table}

\begin{table}[!ht]
\centering
\resizebox{0.7\columnwidth}{!}{%
\begin{tabular}{l|ccc|ccc}
\hline
\multirow{2}{*}{Method} & \multicolumn{3}{c}{$D_1$}                         & \multicolumn{3}{c}{$D_2$}                         \\
                        & \multicolumn{1}{l}{50} & \multicolumn{1}{l}{100} & \multicolumn{1}{l}{500} & \multicolumn{1}{l}{500} &
                        \multicolumn{1}{l}{1000}    &
                        \multicolumn{1}{l}{5000} \\
\hline
\ecl     & 0.0356 & 0.0777 & 0.4496 & 0.0242 & 0.0744 & 0.6664  \\
\dlip   & 0.8774 & 0.9087 & 0.9788  & 0.9719 & 0.9870 & 0.9984  \\
\hline
\end{tabular}
}
\caption{\small{Quality of solution, $Q(\lambda)$, while on a time budget.}}
\label{tab:quality-results}
\end{table}

Table~\ref{tab:quality-results} shows a comparison between \dlip - which uses the efficient projection algorithm, the adaptive smoothing method and LBFGSB as the optimizer - and the best performing version of \ecl (with $0.1 < \gamma < 0.001$). This experiment is designed to mimic practical scenarios where one has a fixed time budget to run the solver and use the solution to make decisions about the marketplace. It is easy to see that even in extreme scale real-world marketplace data ($D_1$), in $100$ iterations \dlip gets to a solution that is less than $10\%$ off from the best but \ecl is greater than $92\%$ off the best.

\cite{basu2020} show that commercial solvers (SDPT3, CPLEX, CLP, GUROBI) do not scale to the problem-sizes in web-scale marketplaces and use a distributed version of the Splitting Conic Solver (\scs)~\cite{scs} to establish a baseline for scale. We benchmark \dlip against \ecl and \scs in Table~\ref{tab:scale-results} on real data to show a $20$x improvement over the state-of-the-art. \ecl and \dlip exploit the data sparsity in the constraint matrix ($A$) often present in marketplace data unlike \scs and other commercial solvers. Additionally, \dlip benefits from the global inference algorithms discussed in \S\ref{sec:projection}, \S\ref{sec:gamma}.

\vspace{-0.1cm}
\begin{table}[!ht]
    \centering
    \resizebox{0.6\columnwidth}{!}{%
    
    \begin{tabular}{|l|c|c|c|c|} 
\hline
\multirow{2}{*}{Problem} & \multirow{2}{*}{Scale $n$} & \multicolumn{3}{c|}{Time (hr)}\\
 && \dlip & \ecl & \scs \\
\hline
\multirow{3}{10em}{Email Optimization \cite{basu2020} $nnz(A) = 10I \approx 1B$} & $10^7$ & 0.05 & 0.8 & 2.0\\
& $10^8$ & 0.07  & 1.3 & >24 \\ 
& $10^9$ & 0.20 & 4.0 & >24 \\ 
\hline
\multirow{3}{10em}{Item Matching \eqref{eq:marketplace} $nnz(A) = 100 I \approx 10B $} & $10^{10}$ & 0.25 & 4.5 & >24\\
& $10^{11}$ & 0.60 & 7.2 & >24  \\ 
& $10^{12}$ & 1.60 & 11.9 & >24 \\ 
\hline
    \end{tabular}
}
    \caption{\small{Run time (hrs) for extreme-scale problems on real data. Here, $nnz(A)$ denotes the number of non-zero entries in $A$ and all runs are on Spark $2.3$ clusters with up to $800$ executors.}}
    \label{tab:scale-results}
    %\vspace{-0.4cm}
\end{table}
