# Supplementary material for: Efficient Vertex-Oriented Polytopic Projection for Web-scale Applications
Source: arXiv:2103.05277 source file (2022-01-06)
Supplement: Supplementary file 4 [file infeas.tex]

\section{Infeasibility checking}
\label{app:infeas}

One possibility that we haven't discussed in the paper is that the primal problem (\ref{eq:qp}) can be infeasible, in which case, $g_\gamma^* = \max_{\lambda\ge 0} g_\gamma(\lambda) = \infty$. For each constraint type $\C_i$, it is easy to calculate a bound $B$ such that $\max_{x_i\in\C_i} (c_i^Tx_i + \frac{\gamma}{2} x_i^Tx_i) \leq B$. If the primal is feasible, then strong optimality implies that $g_\gamma^* \le IB$. Thus, if, during the optimization, $g_\gamma > IB$, then it guarantees that the primal is infeasible.

In \S\ref{sec:optinfeas} we described a guaranteed way of checking primal infeasibility. However, since $B$ is a poor bound, it may take a large number of iterations for $g_\gamma$ to hit it and decide infeasibility. To make quick and approximate decisions, consider a popular problem class, $\PP$ in which all elements of $(A,b)$ are non-negative. When we work with $\C$ having an equality constraint, e.g., \SE, \BE, it is possible that $\C$ is infeasible for the primal. On the other hand, \SI and \BI are feasible because $x=0$ satisfies all the constraints. Thus, we could relax \SE to \SI or \BE to \BI, maximize $g_\gamma$ to get its maximum value $G$ quickly. Then we can solve with \SE or \BE and, if $g_\gamma$ goes much higher than $G$ then we can decide infeasibility and go back to the formulation to make suitable changes. See figure~\ref{fig:qa_infeasible} for an example.

\begin{figure}[ht]
%\vskip 0.2in
\begin{center}
\centerline{\includegraphics[width=0.7\columnwidth, clip]{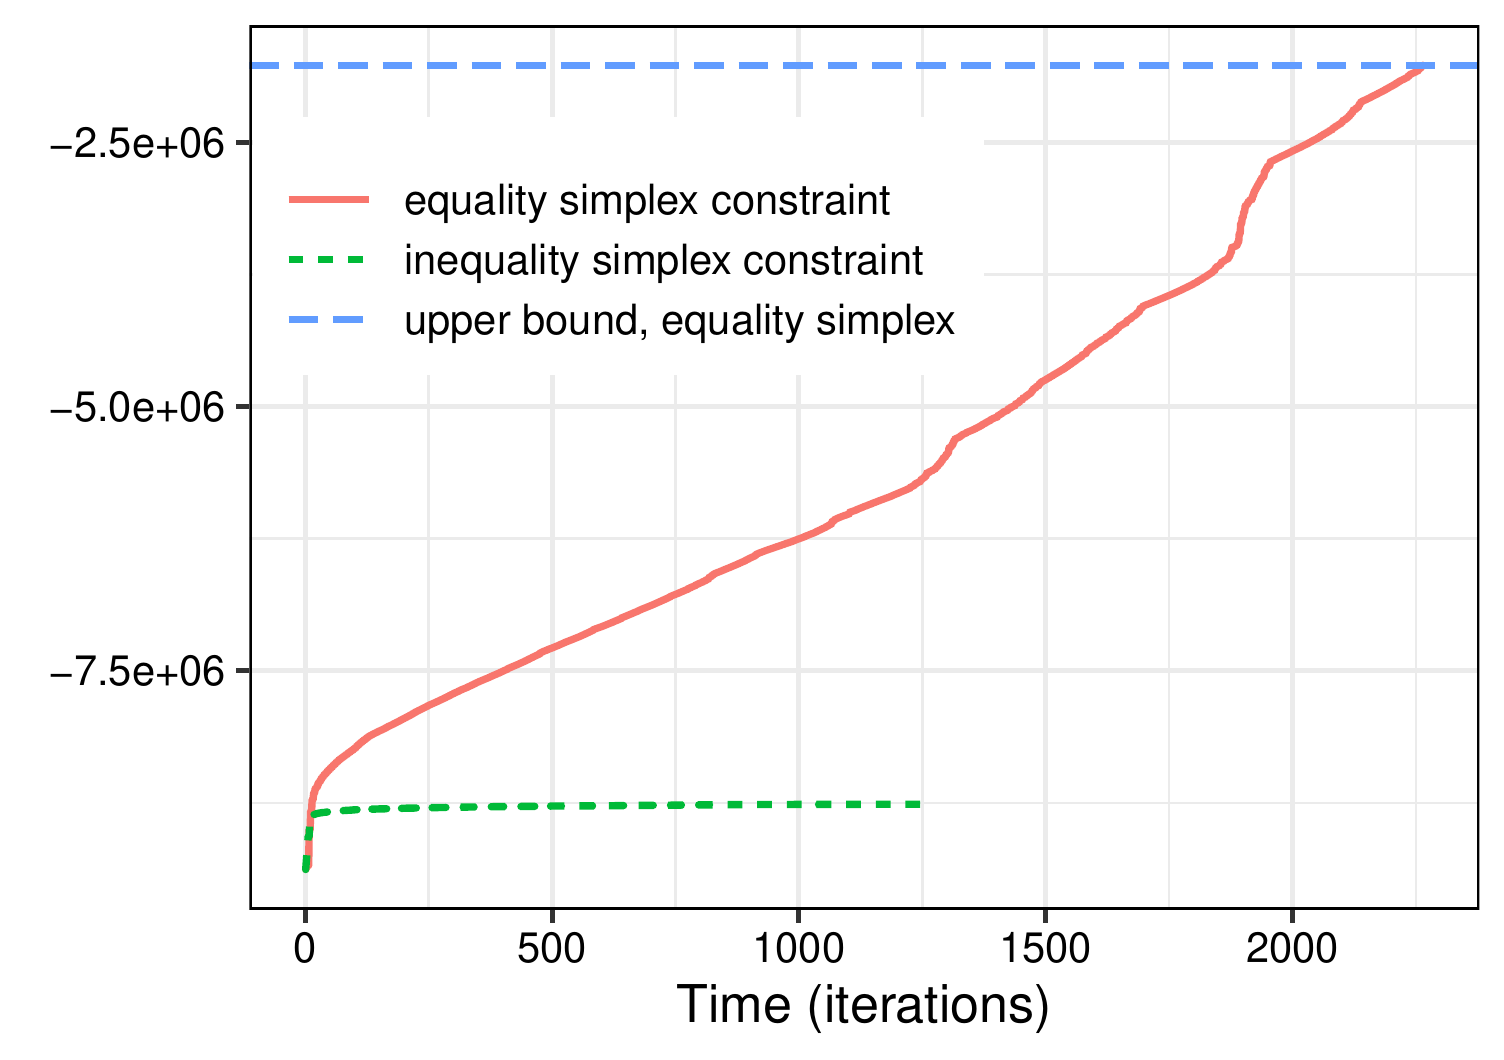}}
\caption{Demonstration of infeasible formulation: unbounded dual function (solid red line) keeps increasing with time, compared to the dual function of a feasible relaxation (dotted green line) that plateaus at its maximum. The top horizontal line (dashed blue) represents the upper bound estimation for the dual. The dual violates the bound and it proves infeasibility.}
\label{fig:qa_infeasible}
\end{center}
%\vskip -0.2in
\end{figure}
