# Supplementary material for: Efficient Vertex-Oriented Polytopic Projection for Web-scale Applications
Source: arXiv:2103.05277 source file (2022-01-06)
Supplement: Supplementary file 5 [file optim.tex]

\section{Optimization}
\label{app:optimization}

%In \S\ref{sec:projection}, we focused on speeding up one evaluation of $(g_\gamma, \nabla g_\gamma)$ by making the inner projection steps very efficient. An orthogonal way of speeding up the solution of (\ref{eq:dual}) is to use better optimization algorithms that reduce the number of $(g_\gamma, \nabla g_\gamma)$ evaluations.

Here we expand over subsection~\ref{subsec:costprofiling} on our discussion of optimization methods.

\ecl~\cite{basu2020} uses the accelerated gradient descent (AGD) method~\cite{nesterov2004introductory} with a fixed step size, $1/L$ where $L$ is a global upper bound on the Lipschitz constant of $\nabla g_\gamma$ that is computed once at the beginning; this computation is also special for $A_i$ matrices with a diagonal structure. The cost of computing the $L$ bound is roughly equal to just a few $(g_\gamma, \nabla g_\gamma)$ evaluations and hence not worrisome. 
This fixed step size works decently  for some problems and datasets.
However, in general, the conservative fixed step size means that the method needs a large number of steps to converge, with each step requiring one $(g_\gamma, \nabla g_\gamma)$ evaluation. The following points are important to note. (a) The bound on $L$ is inversely proportional to $\gamma$ and so, as $\gamma$ becomes small, $L$ becomes large, the fixed step size becomes extremely small and the \ecl method becomes very slow. (b) Lipschitz constant values vary a lot in different parts of the
$(\gamma, \lambda)$ space. For efficient optimization, the right approach is to adapt the step size along the optimization path.

At each optimization iteration, a good optimization method will (a) select a good direction, (b) choose a starting step size, $\eta_0$, and, (c) start from $\eta_0$ and do efficient line-search to obtain the final step size, $\eta$. To get a good $\eta_0$, we devise a heuristic method for estimating the Lipschitz constant.

{\bf Adaptive $\mathbf{L}$ estimation}
Let $H$ be the size of the history (number of previous iterations) we use to estimate the Lipschitz constant for the $t^{th}$ iteration. We use
\begin{equation}
    L_t= \max  \frac{||\nabla g(\lambda_s) - \nabla g(\lambda_{s-1}) ||}{|| \lambda_s - \lambda_{s-1} ||} \biggr\rvert_{s=t}^{t-H}
\end{equation}
The starting step size for the $t^{th}$ iteration, $\eta_0$ is then given by $\eta_0 = \eta_{min}$ if $t \leq H$; and, $\eta_0 = \min (1/L_t, \eta_{max})$ if $t > H$, where $\eta_{min}$ and $\eta_{max}$ are lower and upper bounds on the starting step size.
%We have bounds for min step size $(s_{min} = 1E-5)$ and max step size $(s_{max} = 0.1)$. 

For line-search, the weak Wolfe bisection method~\cite{Burke2018LineSA} starting from $\eta_0$ is suitable for use with a traditional optimization algorithm. 

{\bf Projected Gradient Ascent (PGA)} For solving the constrained maximization problem (\ref{eq:dual}), the simplest method is to use the above adaptive $L$ estimation to get a starting value for the step size, and line-search ideas with projected gradient ascent, in which, at a given $\lambda_t$ with gradient $d_t = \nabla g_\gamma(\lambda_t)$, line search is done along the piecewise linear path, $\lambda(\eta) = \max (\lambda_t+\eta d_t, 0)$ where the $\max$ operation is applied component-wise. 

{\bf LBFGS-B}~\cite{Byrd95alimited-memory} is an even better method for our use. It is a specialized version of LBFGS for problems with bound constraints ($\lambda\ge 0$ in our case).

In the above methods, when we use strong Wolfe's conditions for line search, the method to find the point of sufficient decrease satisfying the strong Wolfe conditions can be unstable as we get close to the true solution\footnote{This can happen due to the fact that $g_0$ is a non-smooth function of $\lambda$ and so $g_\gamma$ can become less smooth as $\gamma$ becomes small.}. Typically, detecting the instability and terminating the line search early gives good results.

%\keerthi{Rohan, what other optimization details do you want to include? LBFGSB line-search issues? Do you want to talk about the lack of ability to know internals such as when an iteration is complete?} \rohan{lets talk about the first and not the second because if we really want it we can achieve the later by not depending on the underlying library like breeze.}

%\keerthi{Include here, any experiments that are not covered in the $\gamma$ tuning section.}

%{\bf Experiment 1}
%Choose a couple of datasets for which we know the true obj fun optimum, say a unit test problem or a decent sized problem that can be solved 
%exactly using SCS. Plot the $\log (g_\gamma(\lambda_\gamma) - g_\gamma(\lambda_t))$ vs number of $g_\gamma$ evaluations. Show AGD-Eclipse, LBFGS-B and PGA as three curves on the same plot. Time to reach $10^-3*gdiff$ can also be shown.

%{\bf Experiment 2} 
%Take three $\gamma$ values - big to small - and show how difficult the problem solution becomes as $\gamma$ becomes small. We can study this for all three methods separately (e.g., for each method, one plot of $(g_\gamma(\lambda_\gamma) - 
%g_\gamma(\lambda_t))$ vs number of $g$ evaluations that overlaps all 3 $\gamma$ solutions) and later decide how to organize the plots compactly. Time to reach $10^-3*gdiff$ can also be shown.

%Write summary conclusions. 
%We should not make any big novelty claim here except say that, the new choices give great improvements over Eclipse.
