# Supplementary material for: Efficient Vertex-Oriented Polytopic Projection for Web-scale Applications
Source: arXiv:2103.05277 source file (2022-01-06)
Supplement: Supplementary file 6 [file qlambda.tex]

{\large\bf Correction of an error in the paper}

In \S\ref{sec:experiments} we defined the quality of solution as
\begin{equation}
  Q(\lambda) = 
  %\frac{(\gbest - g_0(\lambda))}{(\gbest - g_0(0))}
  \frac{\gtil_0 - g_0(\lambda)}{\gtil_0 - g_0(0)}
  \label{qlambda:quality}
\end{equation}
There is a typo in this definition. The correct definition is
\begin{equation}
  Q(\lambda) = 
  %\frac{(\gbest - g_0(\lambda))}{(\gbest - g_0(0))}
  \frac{\gtil_0 - g_0(0)}{\gtil_0 - g_0(0)}
  \label{qlambda:quality1}
\end{equation}
All quality numbers in Figure~\ref{fig:gamma-results} (\S\ref{sec:gamma}),
Figure~\ref{fig:opt-results} (\S\ref{sec:experiments}), 
and Table~\ref{tab:quality-results} (\S\ref{sec:experiments})
use this $Q(\lambda)$ definition in (\ref{qlambda:quality1}). 
This score approximates the true quality defined by
\begin{equation}
  Q^*(\lambda) = 
  %\frac{(\gbest - g_0(\lambda))}{(\gbest - g_0(0))}
  \frac{\gtil_0 - g_0(\lambda)}{g_0(\lambda_0) - g_0(0)}
  \label{qlambda:qualitytrue}
\end{equation}
{\it Iterations} in the horizontal axis in Figures~\ref{fig:gamma-results} and \ref{fig:opt-results} denotes the number of calls to the gradient of $g_\gamma$.
